# Supplementary material for: Mitigating Popularity Bias in Recommendation with Unbalanced Interactions: A Gradient Perspective
Source: arXiv:2211.01154 source file (2022-10-31)
Supplement: Supplementary file 1 [file supplementary_materials.tex]

\section{supplementary}
\subsubsection{ \textbf{A revisit of BCE loss}}
Binary Cross-Entropy derives a multinomial distribution $p$ over each category from the model outputs $\hat{y}_{ui}$ in RS, and then computes the cross-entropy between the estimated distribution $p$ and ground truth distribution of $y_{ui}$. The Binary cross-entropy loss $L_{BCE}$ can be formulated as:
\begin{equation}
    L_{BCE} = \sum_{(u,i) \in D}  -y_{ui}\, \log(\hat{y}_{ui}) - (1-y_{ui})\:\log(1-\hat{y}_{ui})
\end{equation}

The derivative of the BCE loss with respect to the predicted interaction $\hat{y}_{ui}$ has the following formulation:
\begin{equation}
\begin{aligned}
\frac{\partial \; L_{BCE}}{\partial \; \hat{y}_{ui}}
=
\left\{\begin{matrix}
 p_j-1, & y_{ui} = 1\\
p_j, & y_{ui} = 0\end{matrix}\right.
\end{aligned}
\end{equation}

\textcolor{red}{
For the optimization of BCE, similar to BPR loss, we notice that for a popular item $i$ which often appears in observed interactions, it can also be taken as a negative sample for a non-observed interaction. So the non-observed interaction category $y=0$ will lead to a discouraging gradient $p_j$ for model updating, which further leads the RS model to predict low probability for the category $y=0$. If j is a rare category, the discouraging gradients will occur much more frequently than encouraging gradients 
in the iterations of optimization. The accumulated gradients will have a non-negligible impact on that category. Finally, even positive samples for category j might get a relatively low probability from the model.
}
